# Supplementary material for: Perfect Match: A Simple Method for Learning Representations For Counterfactual Inference With Neural Networks
Source: arXiv:1810.00656 source file (2019-05-27)
Supplement: Supplementary file 1 [file appendix.pdf]

# Supplementary Material for: Perfect Match: A Simple Method for Learning Representations For Counterfactual Inference With Neural Networks

**Patrick Schwab**[1], **Lorenz Linhardt**[2], **Walter Karlen**[1]
[1]Institute of Robotics and Intelligent Systems, ETH Zurich, Switzerland
[2] Department of Computer Science, ETH Zurich, Switzerland
patrick.schwab@hest.ethz.ch

## A Precision in Estimation of Heterogenous Effect (PEHE)

When the underlying noiseless distributions $\mu_j$ are not given, PEHE is calculated using:

$$\hat{\epsilon}_{\text{PEHE}} = \frac{1}{N}\sum_{n=0}^{N}\Big([y_1(n) - y_0(n)] - [\hat{y}_1(n) - \hat{y}_0(n)]\Big)^2 \tag{A.1}$$

## B Average Treatment Effect (ATE)

The ATE measures the average difference in effect across the whole population (Hill 2011). It can be useful indicator of how well an ITE estimator performs at comparing two treatments across the entire population.

$$\epsilon_{\text{ATE}} = ||\frac{1}{N}\sum_{n=0}^{N}\mathbb{E}_{y(n)\sim\mu(n)}[y(n)] - \frac{1}{N}\sum_{n=0}^{N}\hat{y}(n)||_2^2 \tag{B.1}$$

Similar to Equation (A.1), the counterfactual treatment effect can be estimated using the noisy ground truth outcomes if the underlying noiseless distributions $\mu_j$ are not given:

$$\hat{\epsilon}_{\text{ATE}} = ||\frac{1}{N}\sum_{n=0}^{N}y(n) - \frac{1}{N}\sum_{n=0}^{N}\hat{y}(n)||_2^2 \tag{B.2}$$

## C Consistency of Perfect Match

*Proof of Theorem 1.*

$$\lim_{N\to\infty} \mathbb{E}(\hat{f}(x)|X, T=t) = \lim_{N\to\infty} \mathbb{E}(\hat{Y}|X, T=t) \quad \text{(Definition of } \hat{Y}\text{)}$$
$$= \lim_{N\to\infty} \mathbb{E}(\hat{y}_t|X, T=t) \quad \text{(}T=t\text{ and independent heads)}$$
$$= \lim_{N\to\infty} \mathbb{E}(\hat{y}_t|X) \quad \text{(Conditional independence assumption (1))}$$

Although the PM algorithm adapts SGD to optimise $\begin{cases} \text{MSE}(\hat{y}_t, y_t) & \text{if } t \text{ is factual} \\ \text{MSE}(\hat{y}_t, y_{\text{NN}_t}) & \text{if } t \text{ is counterfactual} \end{cases}$

we can subsume this conditional statement as a single nearest neighbour estimate $\text{NN}_t$ treated with treatment $t$ for which we are guaranteed to have access to a perfect match, i.e. an exact nearest neighbour with $X = x$ and $T = t$ if we are balancing on the covariates or in terms of the propensity score $p(t|X)$ if we are balancing on treatment propensity, for observed factual outcomes. Under the assumption of convergence at the training data we then have

$$= \lim_{N\to\infty} y_{\text{NN}_t} \quad \text{(Convergence in objective)}$$
$$= y_t \quad \text{(Smoothness assumption, and consistency of NN)}$$

since nearest neighbour estimators are consistent.

□

## D Implementation Details Perfect Match

We trained a Support Vector Machine (SVM) with probability estimation as propensity score estimator $E_{\text{PS}}$. To speed up recalling nearest neighbours, we additionally prepared an index per treatment into $X_{\text{train}}$ sorted by propensity score. At augmentation time, we used binary search on this index to find the nearest neighbours by propensity score in O(log $N_t$) where $N_t$ is the number of samples $X$ in $X_{\text{train}}$ assigned to the treatment group $t$. To avoid overfitting to specific edge samples when propensity scores are not distributed evenly in the training set, we chose at random from one of the $k$=6 closest samples by propensity score. See Table S1 for a comparison of the effects on predictive performance of choosing varying values of $k$. For the "+ on $X$" model we matched, using the Euclidean distance, directly on the covariates $X$ on IHDP, and using a low dimensional representation of $X$, obtained using principal component analysis (PCA) with 50 principal components, on News.

Table S1: Comparison of PM with varying numbers of nearest neighbours $k$ considered for randomised matching on the News-2/4/8/16 datasets ($k$=1 corresponds to no randomisation; $k$=6, in cursive, are the results reported in the main body). We report the mean value ± the standard deviation of $\sqrt{\hat{\epsilon}_{\text{PEHE}}}$ on the test sets over 50 runs. There was no significant differences between different levels of $k$ and $k$=6 (significance level $\alpha < 0.05$). In particular, there was no significant difference between using randomisation and not using randomisation.

| Method | News-2 $\sqrt{\hat{\epsilon}_{\text{PEHE}}}$ | News-4 $\sqrt{\hat{\epsilon}_{\text{PEHE}}}$ | News-8 $\sqrt{\hat{\epsilon}_{\text{PEHE}}}$ | News-16 $\sqrt{\hat{\epsilon}_{\text{PEHE}}}$ |
|---|---|---|---|---|
| PM ($k$=1) | 16.79 ± 1.16 | 21.86 ± 2.24 | 20.70 ± 1.87 | **20.06** ± 1.43 |
| PM ($k$=3) | 16.82 ± 1.17 | 21.49 ± 2.43 | **20.50** ± 1.48 | 20.28 ± 1.52 |
| *PM ($k$=6)* | **16.76** ± 1.26 | 21.58 ± 2.58 | 20.76 ± 1.86 | 20.24 ± 1.46 |
| PM ($k$=9) | 16.91 ± 1.18 | 21.56 ± 2.58 | 20.75 ± 1.53 | 20.47 ± 1.94 |
| PM ($k$=12) | 17.11 ± 0.94 | 21.16 ± 2.20 | 21.10 ± 2.14 | 20.28 ± 1.64 |
| PM ($k$=15) | 16.87 ± 1.14 | **20.94** ± 2.05 | 20.92 ± 1.80 | 20.48 ± 1.80 |

# E Reduced Variance is Linked to Improved Performance in Estimating Treatment Effects

In the standard supervised setting, the variance added by minibatch SGD leads to slower convergence (Csiba & Richtárik 2018), but will not typically lead to models that perform worse if they are trained until a convergence criterion has been met, e.g. early stopping. It is therefore perhaps surprising that we observe a difference not just in convergence (Figure 6), but also in counterfactual estimation performance (Tables 3 and 4) when comparing models trained with and without batch matching.

A potential cause of the observed difference in treatment effect estimation performance is that we do not have access to the true counterfactual error in observational data to select the best model encountered during training. We therefore have to resort to using the factual error (e.g. factual MSE) or an estimator based on the factual error (e.g. NN-PEHE) to select the best encountered model. However, when the variance during training is high, chances are that we select a model based on the factual error that at this point during the training happens to be suboptimal in terms of counterfactual error. Through this mechanism, added variance during training for counterfactual inference is directly linked to worse expected performance in treatment effect estimation (Figure S1). We do not observe the same behavior in standard supervised learning tasks because we have direct access to the underlying objective, and are therefore able to select the best encountered model regardless of the variance during optimisation, i.e. models that during training do not perform well momentarily will not be selected because their measured error is high. We confirmed experimentally that gradient steps are more likely to be in opposing directions when not using PM (Figure S2).

# F Nearest Neighbour Approximation of PEHE for Multiple Treatments (NN-mPEHE)

The $\hat{\epsilon}_{\text{NN-PEHE}}$ metric can be extended to the multiple treatment setting by considering the mean $\hat{\epsilon}_{\text{NN-PEHE}}$ between all $\binom{k}{2}$ possible pairs of treatments:

$$\hat{\epsilon}_{\text{NN-mPEHE}} = \frac{1}{\binom{k}{2}} \sum_{i=0}^{k-1} \sum_{j=0}^{i-1} \hat{\epsilon}_{\text{NN-PEHE},i,j} \tag{F.1}$$

# G Pseudocode Propensity Score Matching (PSM)

Algorithm S1 outlines the procedure of preprocessing a training set using $\text{PSM}_{\text{MI}}$. For $\text{PSM}_{\text{PM}}$, we used the PM matching algorithm (see Algorithm 1) to find matches between samples from the treatment groups. For $\text{PSM}_{\text{MI}}$, we used the MatchIt package (Ho et al. 2011) on setting "nearest" to find matches between sets of samples from two treatment groups (function `get_matched_samples`).

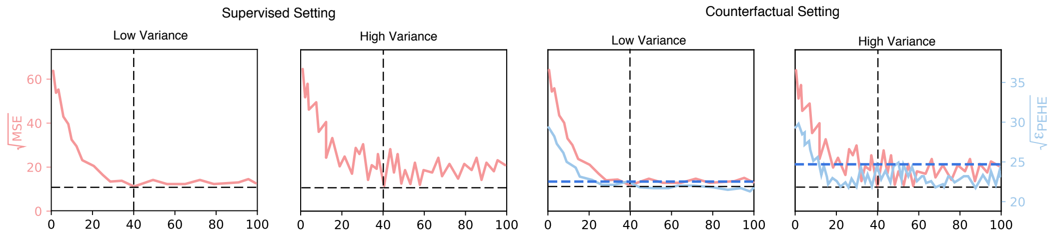


Figure S1: Illustration of the impact of added variance introduced by minibatch SGD during training. In the supervised setting (left), high variance does in general not impact the final performance in terms of expected factual error (red), because we can select (dotted black line) the best encountered model during training using the observed error. In the counterfactual setting (right), we are not able to compute the true counterfactual error (blue) in observational data, and must therefore resort to selecting based on the factual error or a measure derived from the factual error. Even though we encounter models that perform similarly well, we are less likely to select these models under high variance, because we do not have direct access to the counterfactual error and the minimum of the factual error in general does not correspond to the minimum of the counterfactual error, particularly when optimisation of counterfactual and factual error are not well aligned. The dashed blue line indicates the counterfactual error of the model selected based on factual error.

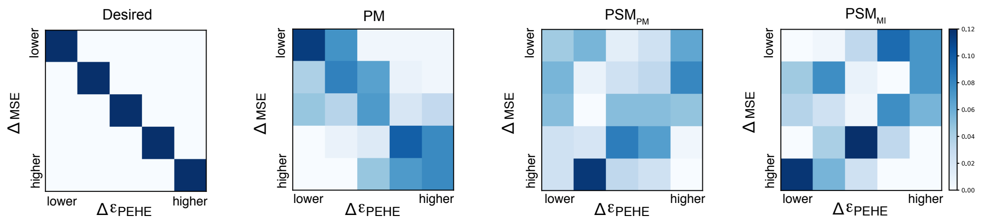


Figure S2: Comparison of the frequencies and magnitudes of individual gradient steps during training of several matching-based methods on the validation set of News-8. The heatmap entries show the frequencies of pairs of differences in factual error ($\Delta$MSE; y-axis) and counterfactual error ($\Delta\epsilon_{\text{PEHE}}$; x-axis) after individual gradient steps. All methods used the same model and only differed in how they addressed treatment assignment bias. The leftmost heatmap shows the desired behavior of gradient steps changing the counterfactual and factual error jointly during training. PM most closely resembles the desired behavior of jointly optimising counterfactual and factual error. In contrast, $\text{PSM}_{\text{PM}}$ and $\text{PSM}_{\text{MI}}$ have a much higher relative frequency of gradient steps that do not move into the same magnitude or direction (off-diagonal entries) for both factual and counterfactual error.

**Algorithm S1** Preprocessing a training set using Propensity Score Matching (PSM). After preprocessing, the training set contains an equal number of samples from each treatment group and the covariates $x_i$ across all treatment groups are approximately balanced.

**Input:** $N$ training samples $X_{\text{train}}$ with assigned treatments $t$, Number of treatment options $k$, function `get_matched_samples` to find nearest matches by propensity score between sets of samples
**Output:** Preprocessed training set $X_{\text{out}}$ consisting of matched samples from each treatment group

**procedure** PREPROCESS_TRAINING_SET:
    $t_{\text{base}} \leftarrow$ index of treatment with smallest number of samples in $X_{\text{train}}$
    $X_{\text{base}} \leftarrow$ all samples in $X_{\text{train}}$ with treatment $t_{\text{base}}$
    **for** $i = 0$ to $k - 1$ **do**
        **if** $i \neq t_{\text{base}}$ **then**
            $X_{\text{current}} \leftarrow$ all samples in $X_{\text{train}}$ with treatment $i$
            $X_{\text{matched}} \leftarrow$ `get_matched_samples`($X_{\text{base}}$, $X_{\text{current}}$)
            Add all samples in $X_{\text{matched}}$ to $X_{\text{out}}$
    Add all samples in $X_{\text{base}}$ to $X_{\text{out}}$

## H TARNET, CFRNET and PD for Multiple Treatments

In TARNET models, we used ELU nonlinearities between the $L$ hidden layers with $M$ hidden units. $L$ and $M$ were hyperparameters that we optimised during hyperparameter optimisation (Section I). We did not use batch normalisation (BN). To extend CFRNET to the multiple treatment setting, we defined the first treatment option as the control treatment and regularised all treatment options to have the same activation distribution in the topmost shared layer (Shalit et al. 2017). For PD, we only used propensity dropout and the propensity estimation network. We did not make use of the alternating training schedule proposed in (Alaa et al. 2017). The "+ MLP" model was a simple MLP with $L$ hidden layers of $M$ hidden units that received the treatment option index $t_j$ as an additional input along with the covariates $X$, and output a $k$-dimensional potential outcome vector $\hat{Y}$. The MLP used ELU nonlinearities between the $L$ hidden layers, and also did not use BN.

## I Hyperparameters

To ensure a fair comparison, we used a standardised approach to hyperparameter optimisation for those methods for which we did not have previously reported performance numbers. In particular, each method we trained was optimised over the same amount of hyperparameter optimisation runs. For the methods that used neural network models (TARNET, CFRNET, PD, $\text{PSM}_{\text{PM}}$, $\text{PSM}_{\text{MI}}$, including "+ on $X$" and "+ MLP", and PM), we chose hyperparameters at random from predefined ranges (Table S2). For CFRNET, we additionally varied the weight of the imbalance penalty at random between 0.1, 1.0, and 10.0. All methods that used a neural network model used the TARNET architecture to

ensure differences in performance are not due to architectural differences. For optimisation, we used the Adam optimiser with a learning rate of $0.001$ for a maximum of 100 (News) or 400 (IHDP) with an early stopping patience of 30 on the factual MSE. We used the default hyperparameters for BART and CF from the "bartMachine" (Kapelner & Bleich 2013) and "grf" (Athey et al. 2016) R-packages. Since CF was designed for estimating the difference in treatment effect between two treatment options and not for estimating treatment outcomes $\hat{y}_t$ directly, we used a baseline ridge regression model with regularisation strength $\alpha = 0.5$ to estimate a control outcome $\hat{y}_0$ for the first treatment and one CF model to estimate the difference in treatment effect between that control treatment and all other treatment options. For GANITE, we used our own implementation since there was no open source implementation available, and - in addition to the parameters in Table S2 - optimised over the supervised loss weights $\alpha$ and $\beta$ (Yoon et al. 2018) between 0.1, 1, and 10. For the GANITE generators and discriminators, we used MLP architectures with $L$ hidden layers of $M$ hidden units each.

Table S2: Hyperparameter ranges used in the performed experiments.

| Hyperparameter | IHDP | News |
|---|---|---|
| Batch size $B$ | 4, 8, 50, 100 | 50 |
| Number of units per hidden layer $M$ | 50, 100, 200 | 40, 60, 80 |
| Number of hidden layers $L$ | 1, 2, 3 | 2, 3 |

## J Computing Infrastructure

We used computing infrastructure consisting of compute nodes with Intel i5 and Xeon CPUs to run the experiments described in this paper.

Table S3: Comparison of methods for counterfactual inference with two and more available treatments on IHDP and News-2/4/8/16. We report the mean value $\pm$ the standard deviation of $\epsilon_{\text{ATE}}$, and $\hat{\epsilon}_{\text{mATE}}$ on the test sets over 1000 and 50 repeated runs for IHDP and News-2/4/8/16, respectively. Best results on each benchmark in bold. $^{\dagger}$ = significantly different from PM ($t$-test, $\alpha < 0.05$).

| Method | IHDP $\epsilon_{\text{ATE}}$ | News-2 $\hat{\epsilon}_{\text{ATE}}$ | News-4 $\hat{\epsilon}_{\text{mATE}}$ | News-8 $\hat{\epsilon}_{\text{mATE}}$ | News-16 $\hat{\epsilon}_{\text{mATE}}$ |
|---|---|---|---|---|---|
| PM | 0.24 $\pm$ 0.20 | **3.99** $\pm$ 1.01 | 10.04 $\pm$ 2.71 | 6.51 $\pm$ 1.66 | 5.76 $\pm$ 1.33 |
| + on $X$ | 0.24 $\pm$ 0.20 | 4.14 $\pm$ 1.27 | $^{\dagger}$ 8.91 $\pm$ 2.00 | **6.36** $\pm$ 1.65 | **5.73** $\pm$ 1.16 |
| + MLP | 0.23 $\pm$ 0.20 | $^{\dagger}$ 5.90 $\pm$ 2.07 | $^{\dagger}$ 14.92 $\pm$ 3.14 | $^{\dagger}$ 14.00 $\pm$ 2.45 | $^{\dagger}$ 16.90 $\pm$ 2.01 |
| kNN | $^{\dagger}$ 3.19 $\pm$ 1.49 | $^{\dagger}$ 7.83 $\pm$ 2.55 | $^{\dagger}$ 19.40 $\pm$ 3.12 | $^{\dagger}$ 15.11 $\pm$ 2.34 | $^{\dagger}$ 17.27 $\pm$ 2.10 |
| $\text{PSM}_{\text{PM}}$ | $^{\dagger}$ 0.34 $\pm$ 0.60 | $^{\dagger}$ 5.02 $\pm$ 2.34 | $^{\dagger}$ 11.62 $\pm$ 2.69 | $^{\dagger}$ 8.81 $\pm$ 1.96 | $^{\dagger}$ 11.04 $\pm$ 2.50 |
| $\text{PSM}_{\text{MI}}$ | $^{\dagger}$ 0.49 $\pm$ 0.81 | $^{\dagger}$ 4.89 $\pm$ 2.39 | $^{\dagger}$ 30.19 $\pm$ 2.47 | $^{\dagger}$ 22.09 $\pm$ 1.98 | $^{\dagger}$ 18.81 $\pm$ 1.74 |
| RF | $^{\dagger}$ 0.64 $\pm$ 1.25 | $^{\dagger}$ 5.50 $\pm$ 1.20 | $^{\dagger}$ 18.03 $\pm$ 3.18 | $^{\dagger}$ 12.40 $\pm$ 2.29 | $^{\dagger}$ 15.91 $\pm$ 2.00 |
| CF | $^{\dagger}$ 0.65 $\pm$ 1.24 | 4.02 $\pm$ 1.33 | $^{\dagger}$ 13.54 $\pm$ 2.48 | $^{\dagger}$ 9.70 $\pm$ 1.91 | $^{\dagger}$ 8.37 $\pm$ 1.76 |
| BART | $^{\dagger}$ 0.53 $\pm$ 1.02 | $^{\dagger}$ 5.40 $\pm$ 1.53 | $^{\dagger}$ 17.14 $\pm$ 3.51 | $^{\dagger}$ 14.80 $\pm$ 2.56 | $^{\dagger}$ 17.50 $\pm$ 2.49 |
| GANITE | $^{\dagger}$ 0.98 $\pm$ 1.90 | $^{\dagger}$ 4.65 $\pm$ 2.12 | $^{\dagger}$ 13.84 $\pm$ 2.69 | $^{\dagger}$ 11.20 $\pm$ 2.84 | $^{\dagger}$ 13.20 $\pm$ 3.28 |
| PD | $^{\dagger}$ 1.37 $\pm$ 1.65 | 4.69 $\pm$ 3.17 | $^{\dagger}$ **8.47** $\pm$ 4.51 | 7.29 $\pm$ 2.97 | $^{\dagger}$ 10.65 $\pm$ 2.22 |
| TARNET | 0.24 $\pm$ 0.29 | $^{\dagger}$ 4.58 $\pm$ 1.29 | $^{\dagger}$ 13.63 $\pm$ 2.18 | $^{\dagger}$ 9.38 $\pm$ 1.92 | $^{\dagger}$ 8.30 $\pm$ 1.66 |
| $\text{CFRNET}_{\text{Wass}}$ | $^{\dagger}$ **0.20** $\pm$ 0.24 | $^{\dagger}$ 4.54 $\pm$ 1.48 | $^{\dagger}$ 12.96 $\pm$ 1.69 | $^{\dagger}$ 8.79 $\pm$ 1.68 | $^{\dagger}$ 8.05 $\pm$ 1.40 |
